# Supplementary material for: Improving Conversational Recommender System via Contextual and Time-Aware Modeling with Less Domain-Specific Knowledge
Source: arXiv:2209.11386 source file (2022-09-23)
Supplement: Supplementary file 1 [file appendix.tex]

\section*{Appendix}
\section{Datasets and Parameter Setting}
\input{tables/data_statistics}
\noindent We first show the basic statistics of the two datasets in \Cref{tab:statistic}. Then we show the detailed parameter search space and best assignment in \Cref{tab:para_setting}. The parameter number of our model is 269M. The training time of one epoch is around 22 minutes when the model is trained an NVIDIA 3090 GPU with a max token number of 4096 and an update frequency of 4. The model needs around 5 epochs to achieve the best performance on the validation set. 

\section{Human Evaluation Details}
We randomly sampled 100 context-response pairs from the test set and collected the corresponding generation results of our models as well as the baseline models. We then employ two crowd-workers to score the results on the scale of [0, 1, 2], where higher scores indicate better quality. Following prior studies, we also evaluate three aspects:
\begin{itemize}[leftmargin=*,topsep=2pt,itemsep=2pt,parsep=0pt]
    \item \textbf{Fluency}: whether a response is in a proper English grammar and easy to understand.
    \item \textbf{Informativeness}: whether a response contains meaningful information. The ``safe responses'' are treated as uninformative as they may be repetitive and meaningless.
    \item \textbf{Coherence}: whether a response is coherent with the context, i.e., the discussion content should be consistent.
\end{itemize}
The scoring details are shown in \Cref{tab:human_eval_scoring} following one of the previous work.

\section{More Analysis}
\paragraph{Limitation of Dist-n Metrics.}
As we find that search strategies seriously affect the Dist-n metrics, we present more analysis on them by setting different values of length penalty (a hyper-parameter that can control the lengths of final generated results) when generating the responses. We display the results of Dist-2 and BLEU2 for EM-TA-BART model with beam search setting in \Cref{fig:limit_distn} (other metrics are in similar trends). We can find that the generated lengths also affect much on the Dist-n, since longer responses allow more different tokens to be generated. However, this is not expected as not the longer the better. Therefore, other metrics including human evaluation are desired to explicitly evaluate generation performance.
\begin{figure}[t]
\caption{\label{fig:limit_distn} Change of Dist-2 and BLEU2 scores when using different length penalty. Larger length penalty ($>1$) indicates allowing generating longer responses.}
\centering
\includegraphics[width=0.45\textwidth]{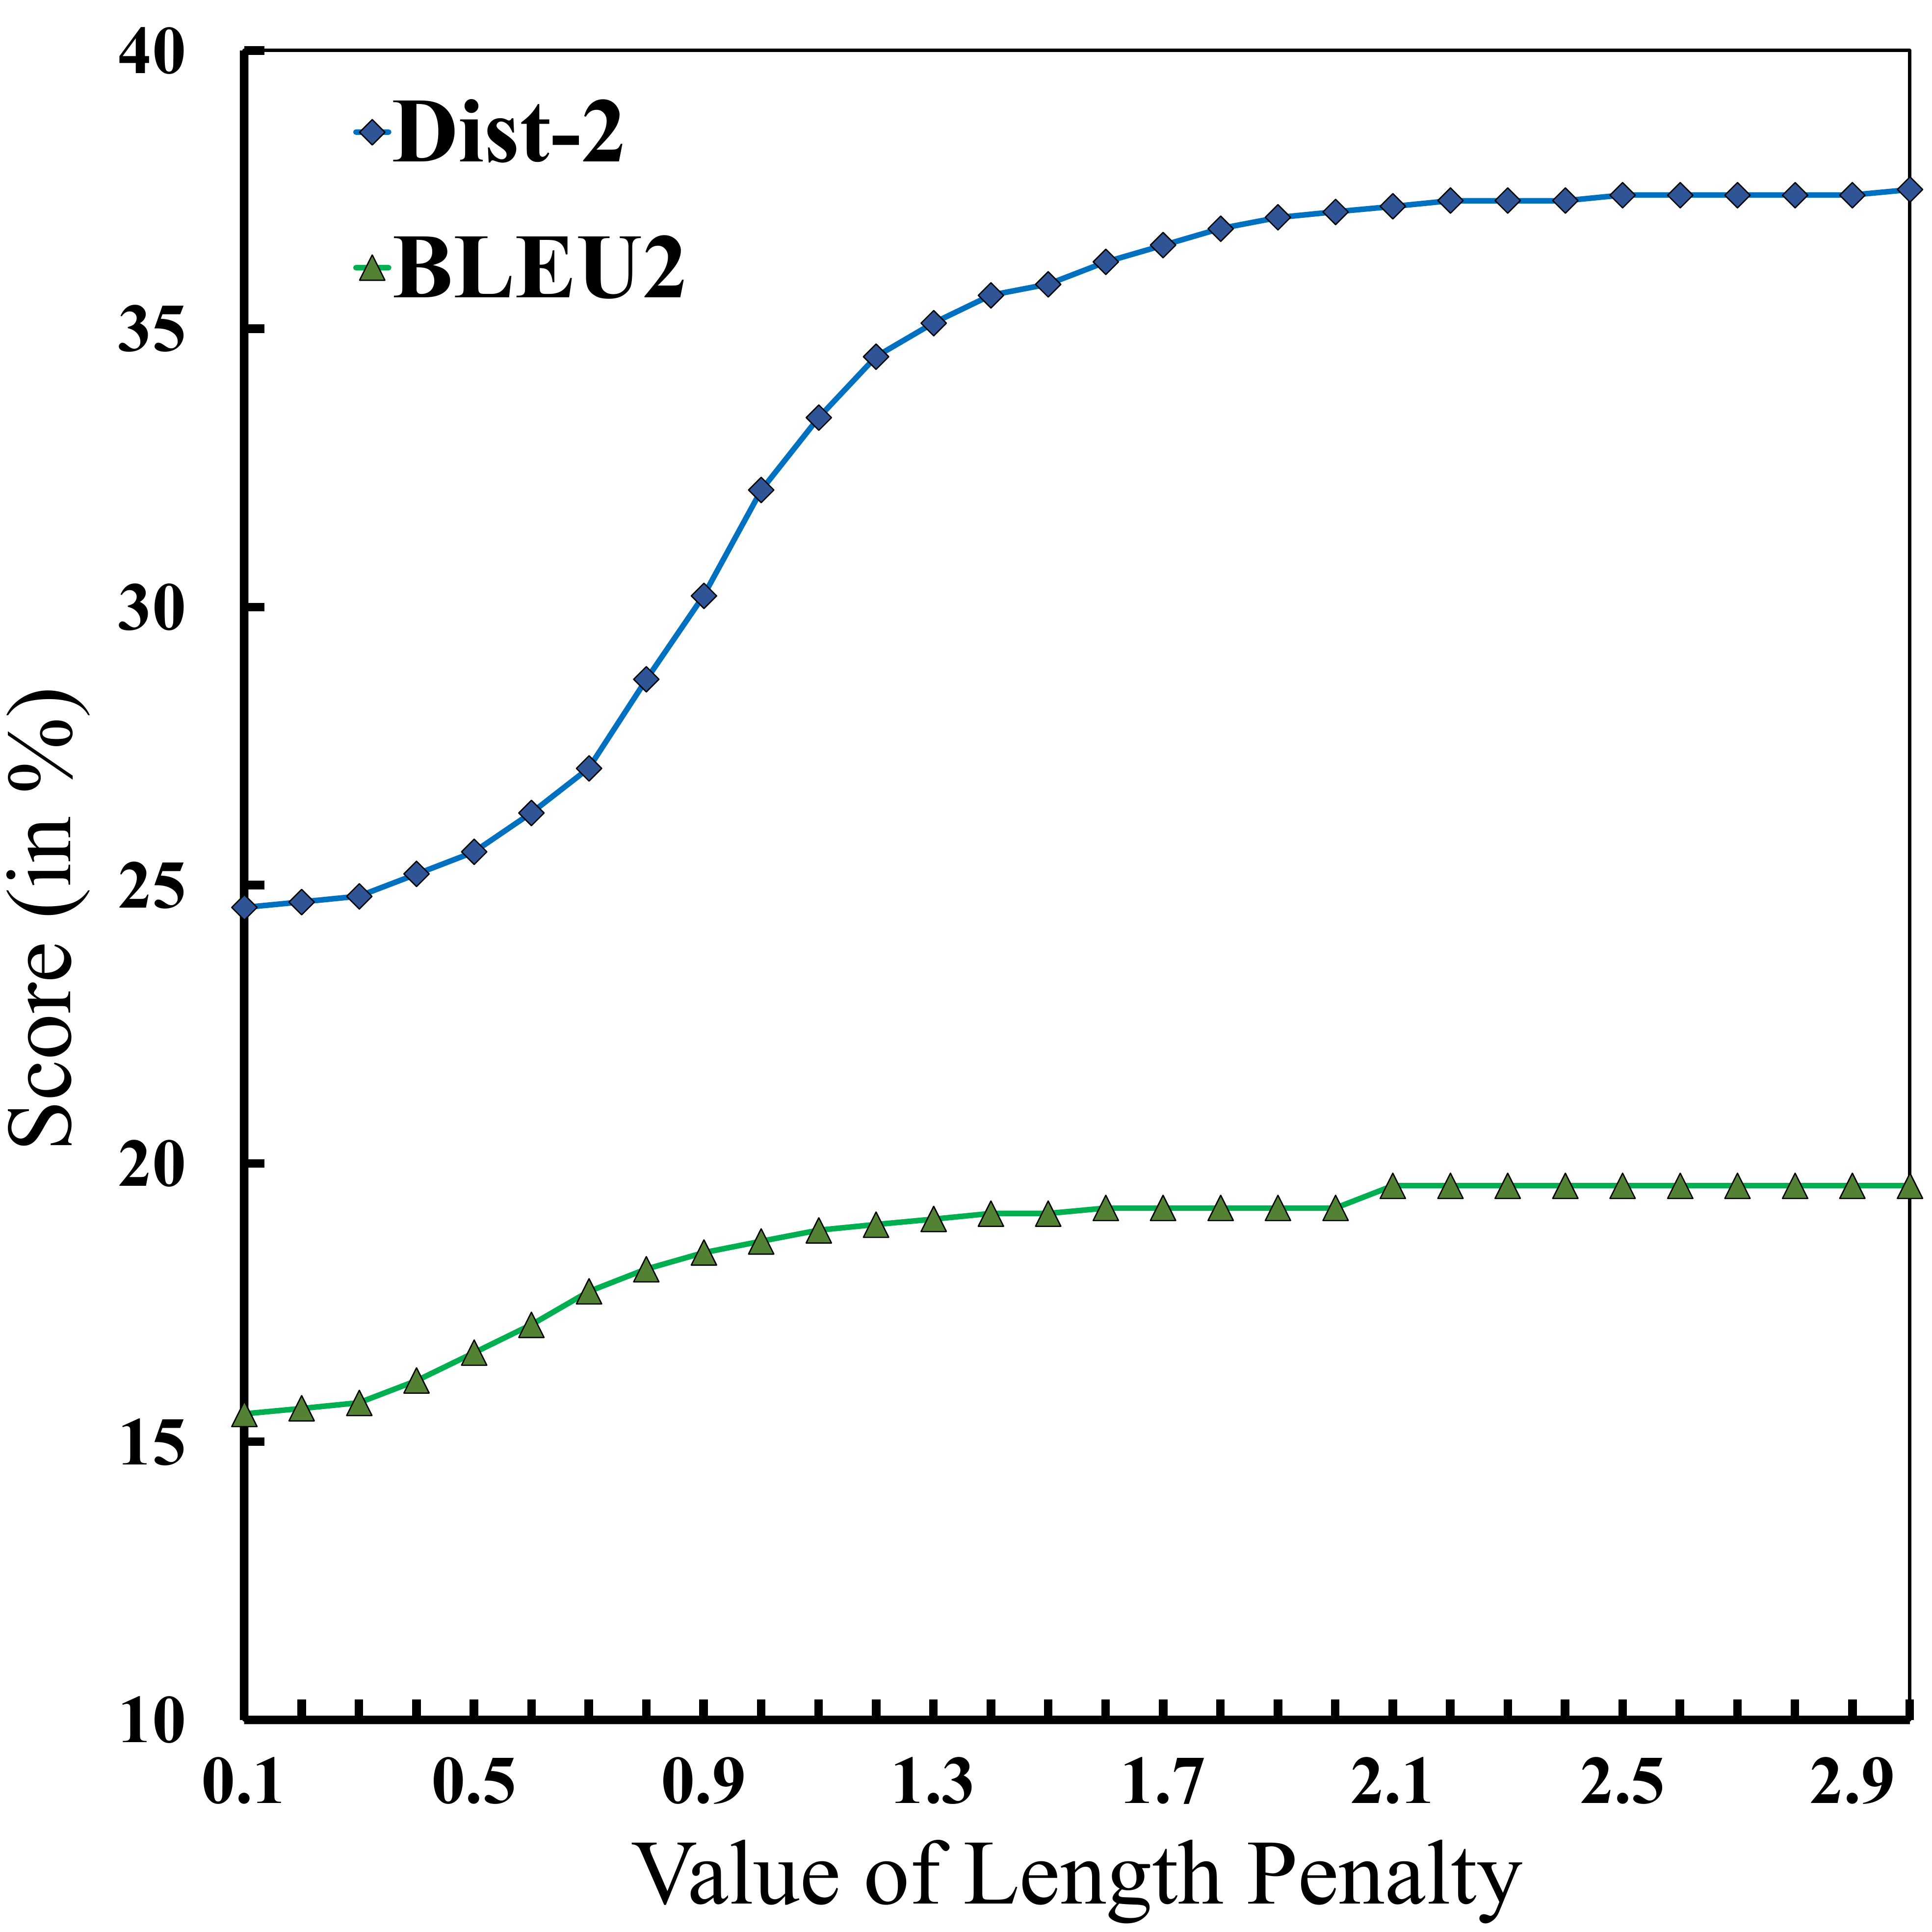}
% \vskip -0.5em

% \vskip -0.5em
\end{figure}

\paragraph{Trade-off between Entity-level and Contextual-level Representations.}
\begin{figure}[ht]
\centering
\includegraphics[width=0.4\textwidth]{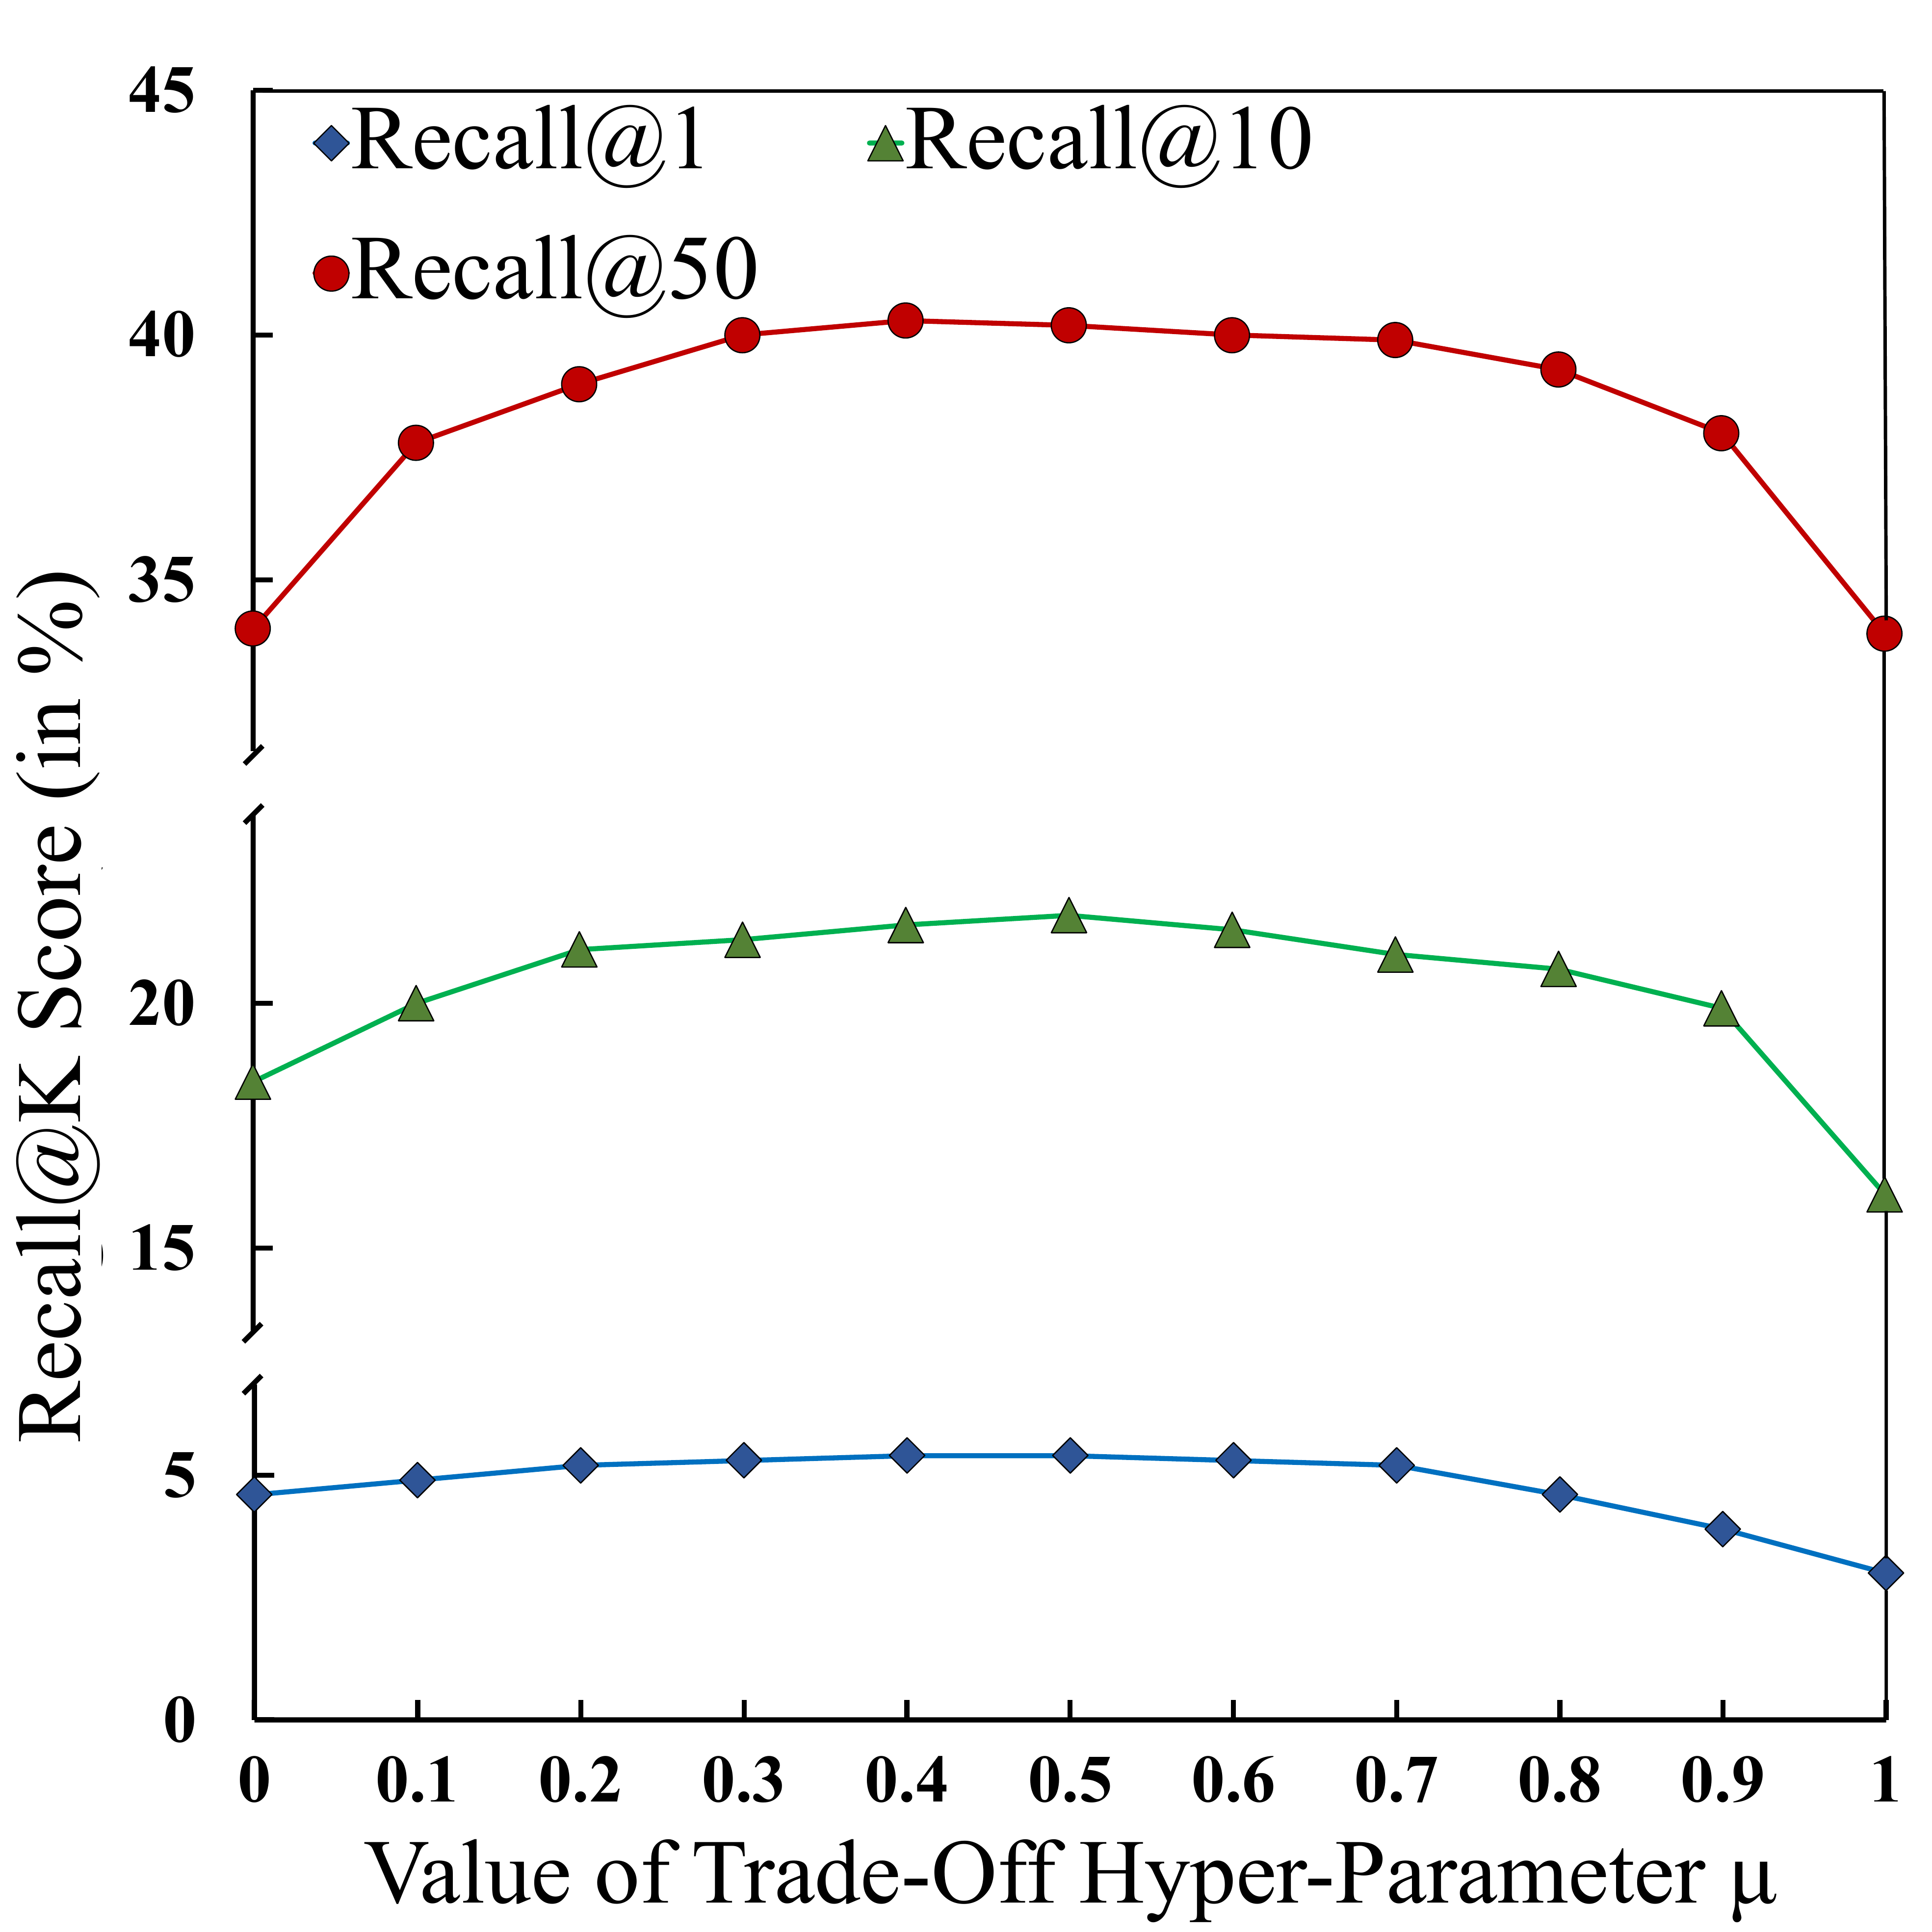}
\vskip -0.5em
\caption{\label{fig:appendix_bias} Change of Recall@1 and Recall@50 scores over different values of trade-off parameter $\mu$.}
% \vskip -1.5em
\end{figure}
We examine the effects of the hyper-parameter $\mu$ in \Cref{eq:rec-joint} by setting its value from 0 (only entity-level representations) to 1 (only contextual-level representations) and display the results of EM-TA-BART model with C+EK input in \Cref{fig:appendix_bias}. As can be seen, Recall@50 is significantly improved when $\mu$ changes from 0 to 0.1 (or 1 to 0.9). This validates that the two representations capture user preferences from a different perspective and can complement each other. The best result is achieved with $\mu=0.5$, showing that both representations are important.

\begin{table}[t]\setlength{\tabcolsep}{1.5mm}
\begin{center}
\begin{tabular}{l|ll}
\toprule[1.0pt]
\textbf{Hyper-parameter}& \textbf{Search Space}  &\textbf{Best} \\
\midrule[0.5pt]
RGCN embedding size & \{128, 256\} &128 \\
RGCN hidden size &\{128, 256\} & 128 \\
RGCN layer number & 1 & 1\\
Normalization factor $Z_{e,r}$ & 1&1 \\
\midrule[0.5pt]
BART layer number &6 &6 \\
BART hidden dim & 768&768 \\
\midrule[0.5pt]
Max token number & \{2048, 4096, 8192, 10240\} &4096 \\
Update frequency & \{1, 2, 4, 8\} & 4\\
LR for recommendation & [1e-4, 2e-4, ..., 8e-3]& 5e-3 \\
LR for generation &[1e-5, 2e-5, ..., 5e-4] &5e-5 \\
Warm-up updates & \{200, 400,..., 2000\} & 1000 \\
Patience & 5 & 5 \\
\midrule[0.5pt]
$\mu$ trade off &[0, 0.1, 0.2, ..., 1.0] & 0.5 \\
\midrule[0.5pt]
beam size & \{2, 4, 6, 8\} & 4 \\
diverse beam group \# & \{2, 4\} & 2\\
length penalty &[0.1, 0.2, ..., 3] & 1.5 \\

\bottomrule[1.0pt]

\end{tabular}
\end{center}
\vskip -1em
\caption{\label{tab:para_setting} Hyper-parameter Search Space and Best Assignment.
}
% \vskip -1.5em
\end{table}

\begin{table}[ht] \setlength{\tabcolsep}{2.4mm}

\begin{center}
\scalebox{0.9}{
\begin{tabular}{c|p{7.5cm}}
\toprule[1.0pt]
\textbf{Score} & \textbf{Fluency} \\
\midrule[0.5pt]
\multirow{2}{*}{\textbf{0}} &The response has many grammar mistakes. \\
 & The response is hard to understand.\\
\midrule[0.5pt]
\multirow{2}{*}{\textbf{1}} & The response has minor grammar mistakes.  \\
& Some part of the response is hard to understand. \\
\midrule[0.5pt]
\textbf{2}& The response is in correct grammar and easy to understand. \\
\bottomrule[1.0pt]
% \hline

\end{tabular}
}
\end{center}

\begin{center}
\scalebox{0.9}{
\begin{tabular}{c|p{7.5cm}}
\toprule[1.0pt] 
% \multicolumn{2}{c}{}  \\
% \hline
\textbf{Score} & \textbf{Coherence} \\
\midrule[0.5pt]
\multirow{4}{*}{\textbf{0}} &  The response is not related with the context.  \\
 & The response simply repeats the context. \\
 & The response has obvious conflicts with the context. \\
\midrule[0.5pt]
\multirow{2}{*}{\textbf{1}} & The response has minor conflicts with the context. \\
& There are some minor logic conflicts in the response. \\
\midrule[0.5pt]
\textbf{2}& The response is coherent with the context. \\
\bottomrule[1.0pt]
% \hline

\end{tabular}
}
\end{center}

\begin{center}
\scalebox{0.9}{
\begin{tabular}{c|p{7.5cm}}
% \hline 
% \multicolumn{2}{c}{}  \\
\toprule[1.0pt]
\textbf{Score} & \textbf{Informativeness} \\
\toprule[1.0pt]
\multirow{4}{*}{\textbf{0}} & The response does not contain any information.  \\
 & This response just repeats the context and fails to bring any additional information.
\\
 & The information is invalid, as the coherence score is 0. \\
\midrule[0.5pt]
\multirow{2}{*}{\textbf{1}} & The information has conflicts with common sense. \\
& There are factual errors in the response. \\
\midrule[0.5pt]
\textbf{2}& The response has appropriate and correct information. \\
\bottomrule[1.0pt]
% \hline

\end{tabular}
}
\end{center}

\vskip -1em
\caption{\label{tab:human_eval_scoring} Scoring details for human evaluation. 
}
% \vskip -1.5em
\end{table}
