# Supplementary material for: Improving Conversational Recommender System via Contextual and Time-Aware Modeling with Less Domain-Specific Knowledge
Source: arXiv:2209.11386 source file (2022-09-23)
Supplement: Supplementary file 2 [file appendix_exp_bias.tex]

\begin{figure}[ht]
\centering
\includegraphics[width=0.4\textwidth]{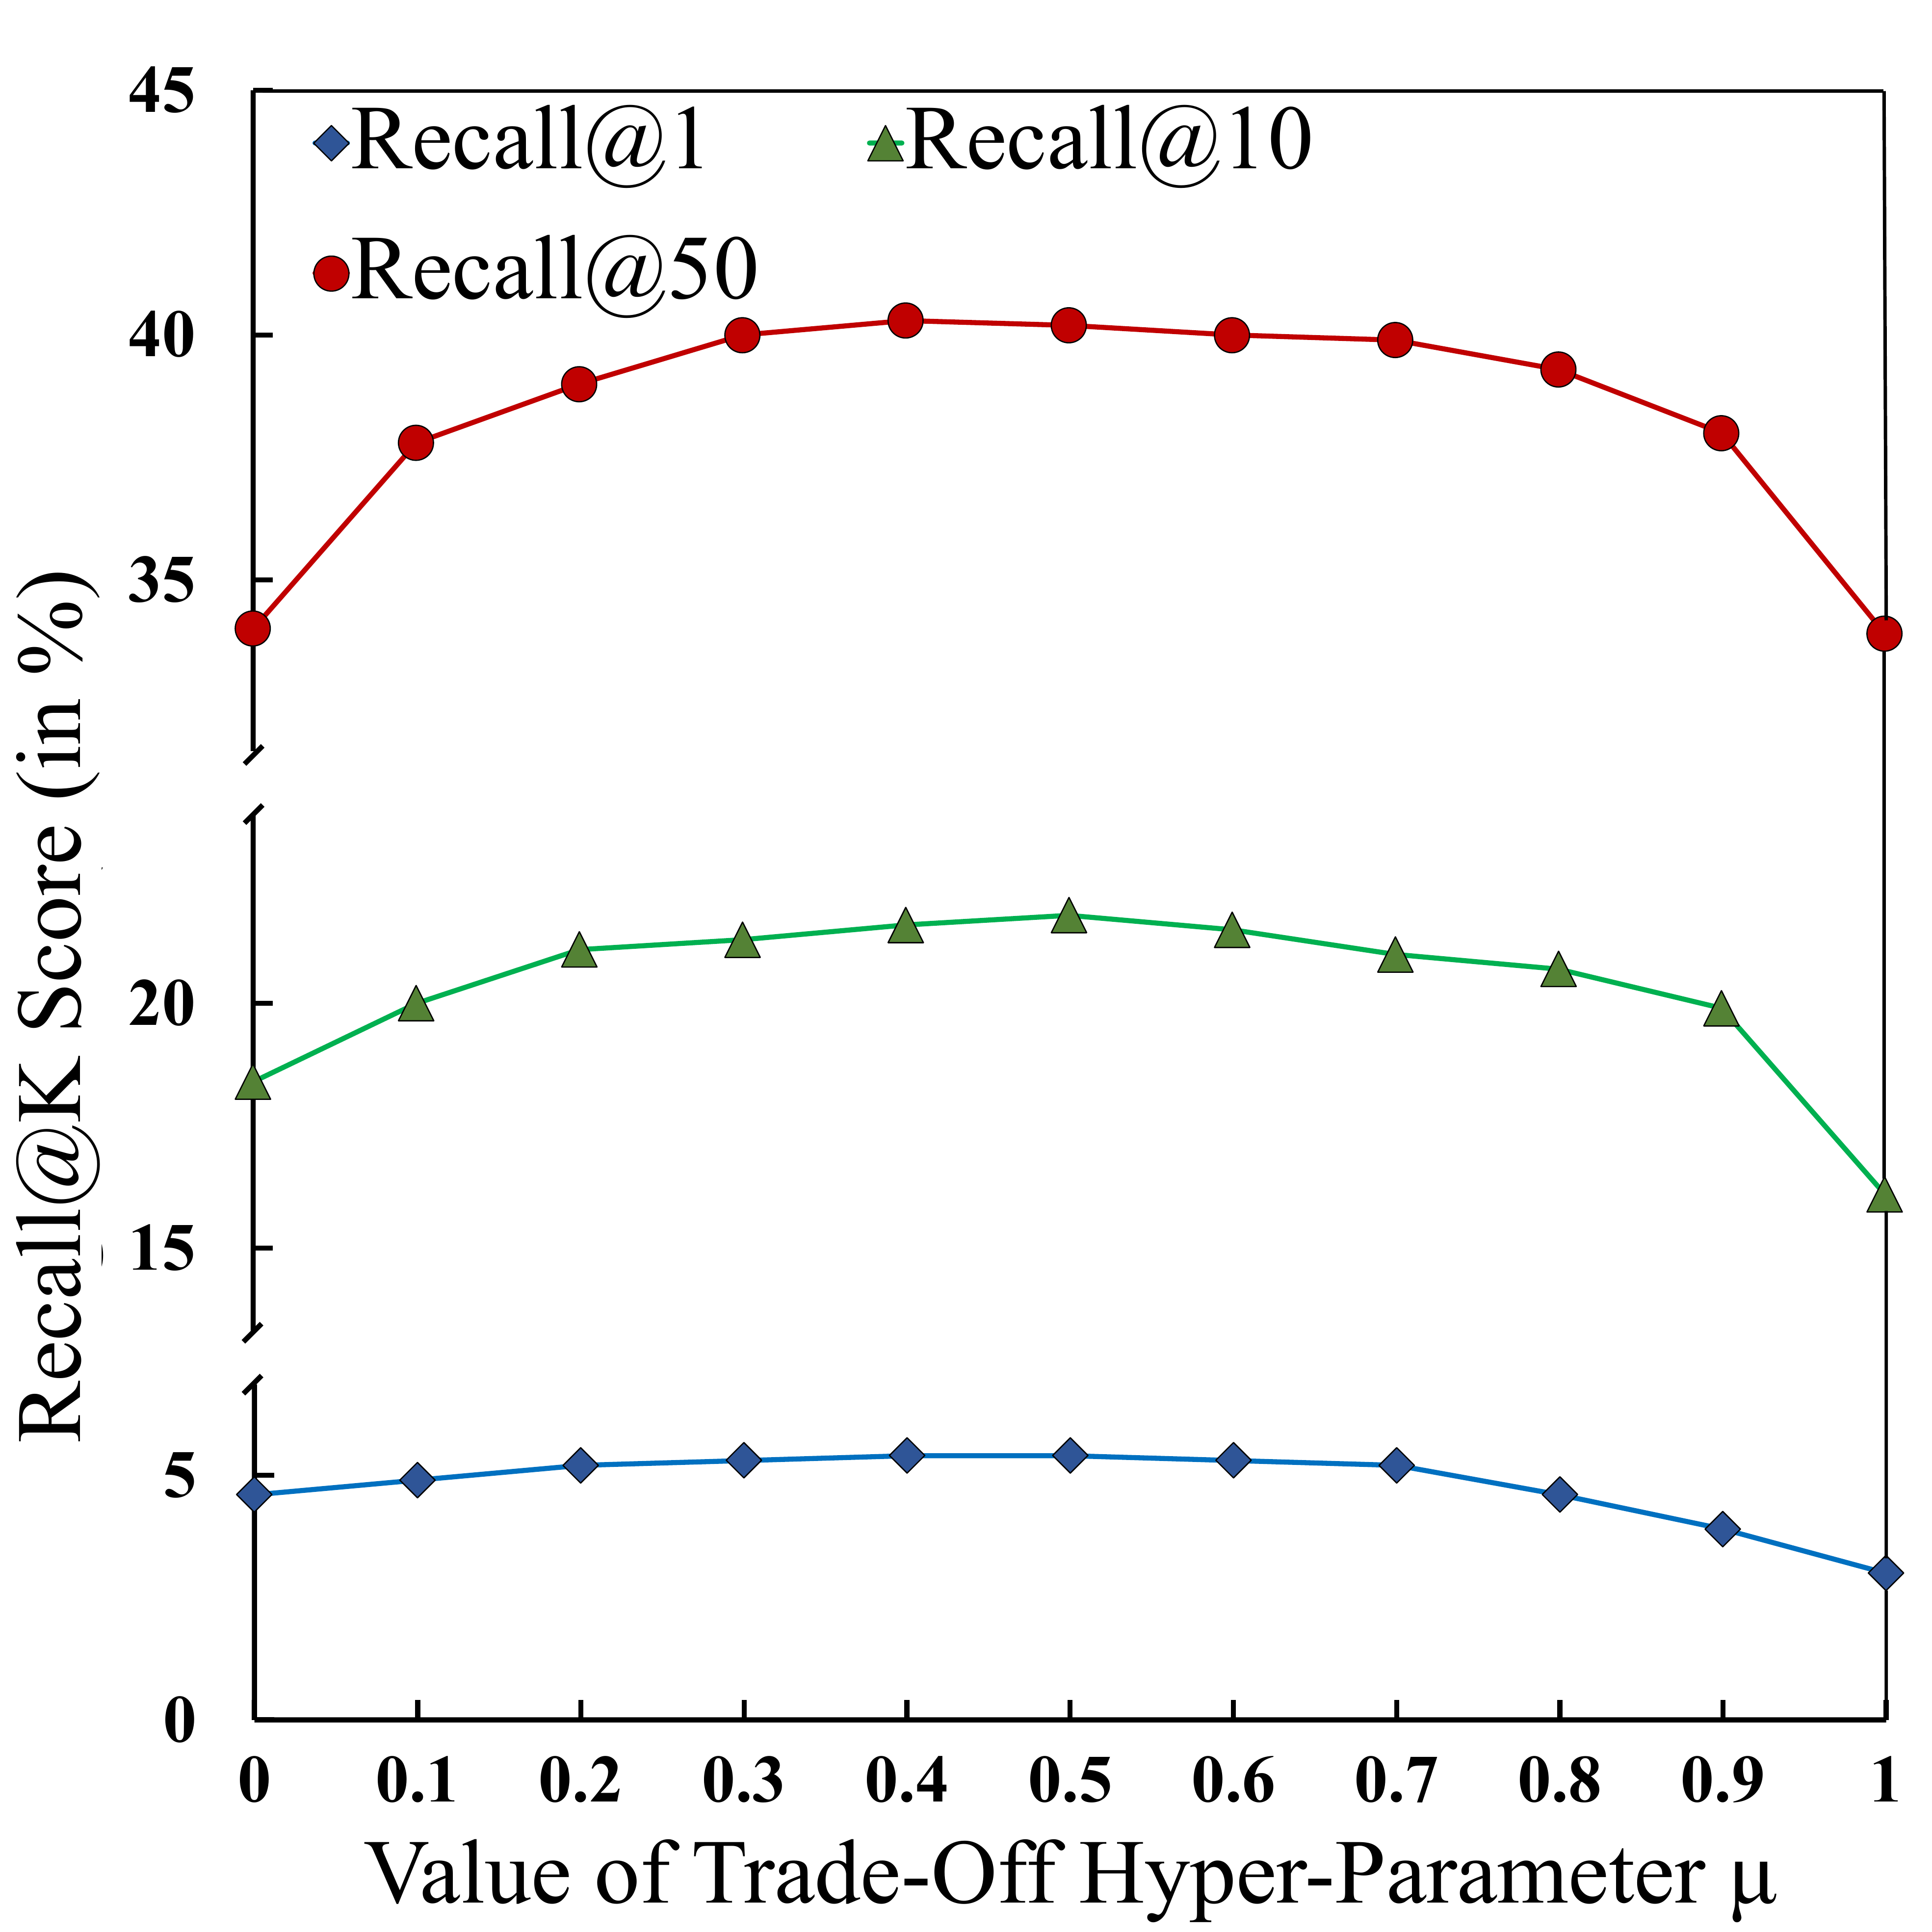}
\vskip -0.5em
\caption{\label{fig:appendix_bias} Change of Recall@1 and Recall@50 scores over different values of trade-off parameter $\mu$.}
% \vskip -1.5em
\end{figure}
