# Supplementary material for: Improving Conversational Recommender System via Contextual and Time-Aware Modeling with Less Domain-Specific Knowledge
Source: arXiv:2209.11386 source file (2022-09-23)
Supplement: Supplementary file 3 [file appendix_human_eval_scoring.tex]

\begin{table}[ht] \setlength{\tabcolsep}{2.4mm}

\begin{center}
\scalebox{0.9}{
\begin{tabular}{c|p{7.5cm}}
\toprule[1.0pt]
\textbf{Score} & \textbf{Fluency} \\
\midrule[0.5pt]
\multirow{2}{*}{\textbf{0}} &The response has many grammar mistakes. \\
 & The response is hard to understand.\\
\midrule[0.5pt]
\multirow{2}{*}{\textbf{1}} & The response has minor grammar mistakes.  \\
& Some part of the response is hard to understand. \\
\midrule[0.5pt]
\textbf{2}& The response is in correct grammar and easy to understand. \\
\bottomrule[1.0pt]
% \hline

\end{tabular}
}
\end{center}

\begin{center}
\scalebox{0.9}{
\begin{tabular}{c|p{7.5cm}}
\toprule[1.0pt] 
% \multicolumn{2}{c}{}  \\
% \hline
\textbf{Score} & \textbf{Coherence} \\
\midrule[0.5pt]
\multirow{4}{*}{\textbf{0}} &  The response is not related with the context.  \\
 & The response simply repeats the context. \\
 & The response has obvious conflicts with the context. \\
\midrule[0.5pt]
\multirow{2}{*}{\textbf{1}} & The response has minor conflicts with the context. \\
& There are some minor logic conflicts in the response. \\
\midrule[0.5pt]
\textbf{2}& The response is coherent with the context. \\
\bottomrule[1.0pt]
% \hline

\end{tabular}
}
\end{center}

\begin{center}
\scalebox{0.9}{
\begin{tabular}{c|p{7.5cm}}
% \hline 
% \multicolumn{2}{c}{}  \\
\toprule[1.0pt]
\textbf{Score} & \textbf{Informativeness} \\
\toprule[1.0pt]
\multirow{4}{*}{\textbf{0}} & The response does not contain any information.  \\
 & This response just repeats the context and fails to bring any additional information.
\\
 & The information is invalid, as the coherence score is 0. \\
\midrule[0.5pt]
\multirow{2}{*}{\textbf{1}} & The information has conflicts with common sense. \\
& There are factual errors in the response. \\
\midrule[0.5pt]
\textbf{2}& The response has appropriate and correct information. \\
\bottomrule[1.0pt]
% \hline

\end{tabular}
}
\end{center}

\vskip -1em
\caption{\label{tab:human_eval_scoring} Scoring details for human evaluation. 
}
% \vskip -1.5em
\end{table}
