# Supplementary material for: Improving Conversational Recommender System via Contextual and Time-Aware Modeling with Less Domain-Specific Knowledge
Source: arXiv:2209.11386 source file (2022-09-23)
Supplement: Supplementary file 4 [file appendix_para_setting.tex]

\begin{table}[t]\setlength{\tabcolsep}{1.5mm}
\begin{center}
\begin{tabular}{l|ll}
\toprule[1.0pt]
\textbf{Hyper-parameter}& \textbf{Search Space}  &\textbf{Best} \\
\midrule[0.5pt]
RGCN embedding size & \{128, 256\} &128 \\
RGCN hidden size &\{128, 256\} & 128 \\
RGCN layer number & 1 & 1\\
Normalization factor $Z_{e,r}$ & 1&1 \\
\midrule[0.5pt]
BART layer number &6 &6 \\
BART hidden dim & 768&768 \\
\midrule[0.5pt]
Max token number & \{2048, 4096, 8192, 10240\} &4096 \\
Update frequency & \{1, 2, 4, 8\} & 4\\
LR for recommendation & [1e-4, 2e-4, ..., 8e-3]& 5e-3 \\
LR for generation &[1e-5, 2e-5, ..., 5e-4] &5e-5 \\
Warm-up updates & \{200, 400,..., 2000\} & 1000 \\
Patience & 5 & 5 \\
\midrule[0.5pt]
$\mu$ trade off &[0, 0.1, 0.2, ..., 1.0] & 0.5 \\
\midrule[0.5pt]
beam size & \{2, 4, 6, 8\} & 4 \\
diverse beam group \# & \{2, 4\} & 2\\
length penalty &[0.1, 0.2, ..., 3] & 1.5 \\

\bottomrule[1.0pt]

\end{tabular}
\end{center}
\vskip -1em
\caption{\label{tab:para_setting} Hyper-parameter Search Space and Best Assignment.
}
% \vskip -1.5em
\end{table}
